# Supplementary material for: Depth Prompting for Sensor-Agnostic Depth Estimation
Source: arXiv:2405.11867 source file (2024-05-20)
Supplement: Supplementary file 1 [file supple_tab_VOID_SUN.tex]

% Please add the following required packages to your document preamble:
% \usepackage{graphicx}
\begin{table*}[ht]
\LARGE
\centering
\resizebox{0.85\textwidth}{!}{%
\begin{tabular}{c||ccc|ccc|ccc|ccc}
\toprule
                        & \multicolumn{3}{c}{VOID 150}                        & \multicolumn{3}{c}{VOID 500}                        & \multicolumn{3}{c}{VOID 1500}                       & \multicolumn{3}{c}{SUN-RGBD}                        \\ 
                        & RMSE            & MAE             & DELTA1          & RMSE            & MAE             & DELTA1          & RMSE            & MAE             & DELTA1          & RMSE            & MAE             & DELTA1          \\ \midrule
CSPN                    & 1.0747          & 0.7991          & 0.2745          & 0.7695          & 0.4776          & 0.4730           & 0.4046         & 0.2121         & 0.7286            & 0.5552          & 0.2464          & 0.8468          \\
NLSPN                   & 0.6964          & 0.5063          & 0.3572          & 0.4672          & 0.2853          & 0.5618          & 0.2563         & 0.1339         & 0.7801            & 0.5910          & 0.2665          & 0.8441          \\
CompletionFormer        & 0.8445          & 0.6976          & 0.2030          & 0.6090          & 0.4447          & 0.3541          & 0.3430         & 0.2158         & 0.5794            & 0.9615          & 0.8574          & 0.0564          \\
Ours                    & \textbf{0.1955} & \textbf{0.1358} & \textbf{0.7243} & \textbf{0.1637} & \textbf{0.1031} & \textbf{0.7457} & \textbf{0.1580} & \textbf{0.098} & \textbf{0.7582}   & \textbf{0.3962} & \textbf{0.2710} & \textbf{0.8402} \\ \bottomrule
\end{tabular}%
}
\vspace{-3mm}
\caption{Quantitative results on VOID and SUN-RGBD dataset.}
\label{tabl:void_sun}
\end{table*}
